# Supplementary material for: Improved anomaly detection by training an autoencoder with skip connections on images corrupted with Stain-shaped noise
Source: arXiv:2008.12977 source file (2020-11-04)
Supplement: Supplementary file 1 [file Appendix.tex]

%%%%%%%%%%%%%%%%%%%%%%%%%%%%%%%%%%%%%%%%%%%%%%%%%%%%%%%%%%%%%%%%%%%%%%%%%%%%%%%%%%%%%%%%%%%
% MODEL SPECIFICATIONS
%%%%%%%%%%%%%%%%%%%%%%%%%%%%%%%%%%%%%%%%%%%%%%%%%%%%%%%%%%%%%%%%%%%%%%%%%%%%%%%%%%%%%%%%%%%

\section{Model specifications}
\label{app:network}

This first appendix aims at providing implementation details of the conducted experiments. We first describe the AESc and AE network architectures and then their training procedure. 

\subsection{CNN architecture}

Our AESc architecture, shown in Figure \ref{fig:architecture}, is a variant of U-net \cite{Ronneberger2015}. AESc takes images of size $256 \times 256$ as input and projects them onto a latent space of $4 \times 4 \times 512$ dimension. The projection towards the lower dimensional space is performed by 6 consecutive convolutional layers strided by a factor 2. The back projection is performed by 6 layers of convolution followed by an upsampling operator of factor 2. All convolutions have a $5 \times 5$ kernel. Unlike the original U-net version, our skip connections perform an addition, not a concatenation, of the feature maps of the encoder to the decoder. 
\begin{figure}[H]
  \centering
  \includestandalone[width=12.5cm]{imgs/Architecture/tikz_architecture}
  \caption{\textbf{AESc architecture performing the projection of an arbitrary image towards the distribution of clean images with the same dimension.} Note that the AE architecture shares the same specifications with the exception of the skip connections that have been removed. }
  \label{fig:architecture}
\end{figure}

\subsection{Training configuration}

All networks have been trained during 250 epochs to minimize the MSE loss over batches constituted of 16 images. We used the Adam optimizer \cite{Kingma2015} with an initial learning rate of 0.01. This learning rate is decreased by a factor of 2 when the PSNR over a validation set constituted of 20\% the corrupted data reaches a plateau for at least 30 epochs. \\
We decided to do not apply data augmentation in the form of vertical and horizontal symmetry or random rotation since we observed that this was detrimental for most of the categories of images. 

%%%%%%%%%%%%%%%%%%%%%%%%%%%%%%%%%%%%%%%%%%%%%%%%%%%%%%%%%%%%%%%%%%%%%%%%%%%%%%%%%%%%%%%%%%%
% NOISE MODELS
%%%%%%%%%%%%%%%%%%%%%%%%%%%%%%%%%%%%%%%%%%%%%%%%%%%%%%%%%%%%%%%%%%%%%%%%%%%%%%%%%%%%%%%%%%%

\section{Impact of the type of noise used as synthetic corruption}

In this paper, we presented one unique model of synthetic corruption, referred to as the Stain model. However, we conducted experiments involving multiple ways of corrupting the training images. This second appendix provides evidence of the supremacy of the Stain model over other models that have been considered. We propose here a fair comparison (using the same network trained with the same procedure) of multiple noise models that can be used to avoid the convergence of the AESc network towards the identity mapping. 

\subsection{Description of the additional noise models}

Ideally, the autoencoder should preserve clean structures while modifying those that are not. Due to the impossibility of collecting pairs of normal and abnormal versions of the same sample, we propose to introduce synthetic corruption during training to explicitly constrain the autoencoder to remove this additive noise. In the paper, we presented the results obtained with our Stain noise model. Besides this Stain model, we also provide here a comparison with three other synthetic noise models represented in Figure \ref{fig:newCorruption}:
\begin{itemize}
\item[] \textbf{Gaussian noise.} Corrupt by adding white noise applied uniformly over the entire image. For normalized intensities between 0 and 1, a corrupted pixel value $x'$, corresponding to an initial pixel value $x$, is the realization of a random variable given by a normal distribution of mean $x$ and variance $\sigma^2$ in the set: $[0.1, 0.2, 0.4, 0.8]$. \vspace*{0.2cm}
%\vspace*{-0.2cm}
%\begin{equation}
%x' = \mathcal{N} \left( x, \sigma^2 \right)
%\end{equation}
%where $\sigma^2$ can take the values  $[0.1, 0.2, 0.4, 0.8]$.
\item[] \textbf{Scratch.} Corrupt by adding one curve connecting two points whose coordinates are randomly chosen in the image and whose color is randomly selected in the gray scale range. The curve can follow a straight line, a sinusoidal wave or the path of a square root function.  \vspace*{0.2cm}
\item[] \textbf{Drops.} Corrupt by adding 10 droplets whose color are randomly selected in the gray scale range and whose shape are circular with a random diameter (chosen between 1 and 2\% of the smallest image dimension). The droplets partially overlap. 
\end{itemize}

\begin{figure}[!ht]
\centering
\begin{minipage}{\linewidth}
      \centering
      \begin{subfigure}{.3\textwidth}
      \centering
        \includegraphics[width=2.2cm]{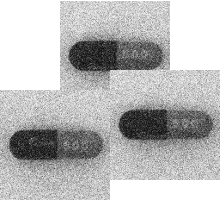}
        \caption{Gaussian noise.}
      \end{subfigure}
       \begin{subfigure}{.3\textwidth}
       \centering
          \includegraphics[width=2.2cm]{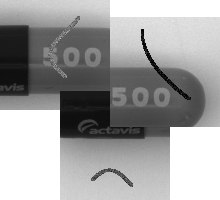}
          \caption{Scratch.}
      \end{subfigure}
       \begin{subfigure}{.3\textwidth}
       \centering
        \includegraphics[width=2.2cm]{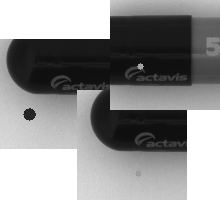}
        \caption{Drops.}
      \end{subfigure}
\end{minipage}
\vspace*{-0.2cm}
\caption{\textbf{Illustration of the Gaussian noise, Scratch and Drops models.} The original clean image is the one seen in Figure \ref{fig:introDiagram}.}
\label{fig:newCorruption}
\end{figure}

In addition, we also considered the possibility to corrupt the training images with a combination of the models introduced previously and the Stain model. We propose two hybrid models:
\begin{itemize}
\item[] \textbf{Structural.} This configuration corrupts training images with a combination of the Stain, Scratch and Drops models. We fix that 60\% of the training images are corrupted with the Stain model while the remaining 40\% are corrupted with the Scratch and Drops models in equal proportions.  \vspace*{0.2cm}
\item[] \textbf{Stain \& Gaussian.} This configuration corrupts training images with a combination of the Stain and the Gaussian noise models. We fix that 60\% of the training images are corrupted with the Stain model while the remaining 40\% are corrupted with the Gaussian noise model.
\end{itemize}

Figure \ref{fig:aesc_corruptionComparison} allows the comparison of the reconstructions obtained for the examples presented previously in the core of the paper with our AESc network trained with different noise models. First, these examples illustrate the convergence of the model towards the identity mapping when the Gaussian noise model is used as synthetic corruption. An analysis of the results obtained over the entire dataset reveals that the AESc + Gaussian noise model does almost not differ from the AESc network trained with unaltered images. \\
Then, we observe that other models improve the identification of defective areas in the images. This is reflected by higher intensities of the reconstruction residual in the defective areas and nearly zero reconstruction residual in the clean areas. With the exception of the Gaussian noise model, the Scratch model is the most conservative, among those considered, in the sense that most of the structures of the input images tend to be reconstructed identically. This practice increases the number of false negative. Also, the Drops model restricts the structures detected as defective to sporadic spots. Finally, the three models based on the Stain noise (Stain, Structural and Stain \& Gaussian) provides the residuals that correlate the most with the segmentation mask. \\

The above observations are consistent with the quantitative performances of the methods. Those results are provided in Tables \ref{table:AESc-residual-image} and \ref{table:AESc-uncertainty-image} (Image-wise detection) and in Tables \ref{table:AESc-residual-pixel} and \ref{table:AESc-uncertainty-pixel} (Pixel-wise detection). The AESc + Stain configuration is the best performing in all use cases when considering the mean performances that are obtained over the entire dataset. The two hybrid models (Structural and Stain \& Gaussian) lead usually to sightly lower performances than those of the Stain model. All other considered models (Drops, Gaussian noise and Scratch) perform worse than the Stain model. \\
Based on these conclusions, we made the choice to present exclusively the Stain noise model in the core of the paper.

\begin{figure}[!ht]
\centering
    \includegraphics[width=12.5cm]{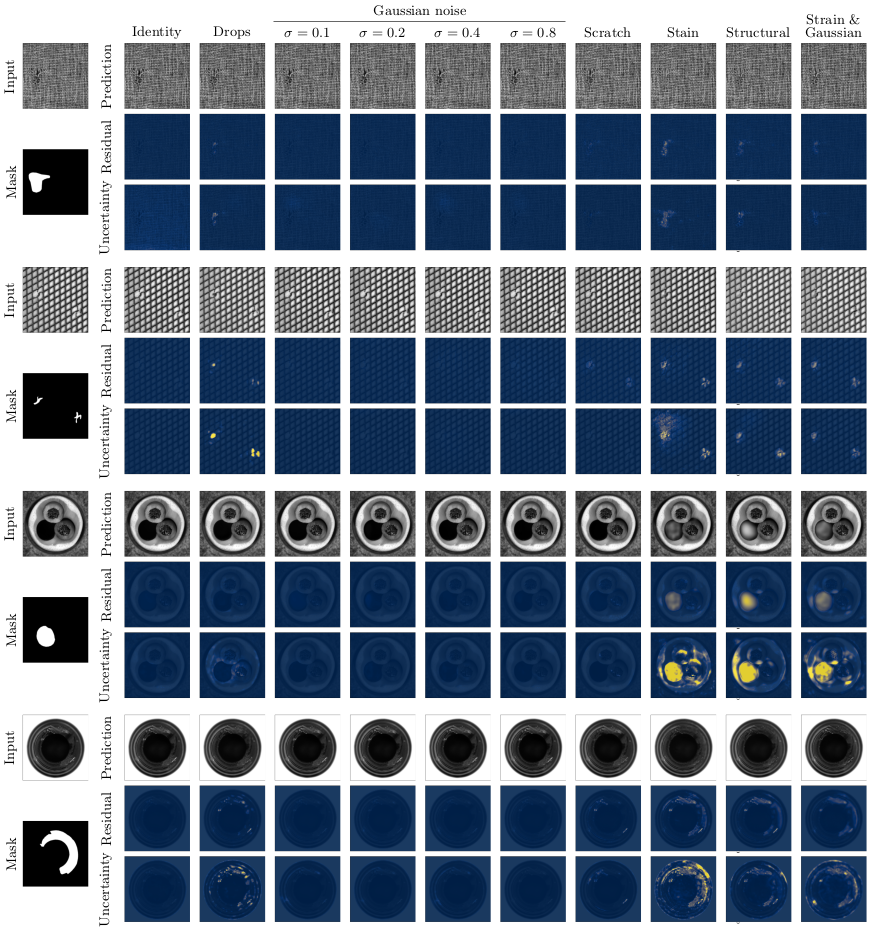}
\caption{\textbf{Predictions obtained with the AESc network trained with different noise models.} Rows and columns are defined as in Figure \ref{fig:qualitativeRes}.} 

\label{fig:aesc_corruptionComparison}
\end{figure}

\newpage
%\subsection{Quantitative results}
\input{Tables/APPENDIX_image-wise}

\tabcolsep=0.03cm

%%%%%%%%%%%%%%%%%%%%%%%%%%%%%%%%%%%%%%%%%%%%%%%%%%%%%%%%%%%%%%%%%%%%%%%%%%%%%%%%%%%%%%%%%%%%%%
% RESIDUAL
%%%%%%%%%%%%%%%%%%%%%%%%%%%%%%%%%%%%%%%%%%%%%%%%%%%%%%%%%%%%%%%%%%%%%%%%%%%%%%%%%%%%%%%%%%%%%%
\begin{table}[!t]
\caption{Pixel-wise AUC obtained with the AESc network trained with different noise models with the residual-based problem formulation. For each row, the best performing approach is highlighted in boldface and the second best is underlined.}
\label{table:AESc-residual-pixel}
\centering
\scriptsize

\resizebox{\textwidth}{!}{

\newcommand\len{0.75}
\newcommand\lenbis{0.55}

\begin{tabularx}{\textwidth}{@{}ll p{\len cm}p{\len cm}p{\lenbis cm}p{\lenbis cm}p{\lenbis cm}p{\len cm}p{\len cm}p{\len cm}p{\len cm}p{\len cm}@{}} 
\arrayrulecolor{black}\cmidrule[0.8pt]{1-12}

& & \multirow{2}{*}{Identity} & \multirow{2}{*}{Drops} & \multicolumn{4}{c}{Gaussian noise ($\sigma$)} & \multirow{2}{*}{Scratch} & \multirow{2}{*}{Stain} & \multirow{2}{*}{Mix1} & \multirow{2}{*}{Mix2} \\

\arrayrulecolor{black!60}\cmidrule(lr){5-8}  

 & &\multicolumn{2}{c}{} & \textbf{$0.1$} & \textbf{$0.2$} & \textbf{$0.4$} & \textbf{$0.8$} & & & &  \\ 

\arrayrulecolor{black}\cmidrule{1-12}

\multirow{5}{*}{\rotatebox[origin=c]{90}{Textures}} & Carpet & 0.52 & 0.68 & 0.50 & 0.50 & 0.50 & 0.50 & 0.62 & \textbf{0.79} & \underline{0.77} & 0.73 \\
& Grid & 0.57 & 0.78 & 0.58 & 0.57 & 0.56 & 0.57 & 0.82 & \textbf{0.89} & 0.86 & \underline{0.87} \\
& Leather & 0.71 & 0.91 & 0.78 & 0.79 & 0.78 & 0.77 & 0.87 & \textbf{0.95} & 0.93 & \underline{0.94} \\
& Tile & 0.62 & 0.60 & 0.58 & 0.58 & 0.58 & 0.60 & 0.60 & \textbf{0.74} & \underline{0.73} & \underline{0.73} \\
& Wood & 0.65 & 0.70 & 0.61 & 0.62 & 0.62 & 0.63 & 0.69 & \textbf{0.84} & \underline{0.81} & 0.78 \\
\arrayrulecolor{black!60}\cmidrule{2-12}
& Mean & 0.61 & 0.73 & 0.61 & 0.61 & 0.61 & 0.61 & 0.72 & \textbf{0.84} & \underline{0.82} & 0.81 \\
\arrayrulecolor{black!60}\cmidrule{1-12}

\multirow{10}{*}{\rotatebox[origin=c]{90}{Objets}} & Bottle & 0.47 & 0.60 & 0.56 & 0.58 & 0.57 & 0.58 & 0.53 & \underline{0.84} & 0.81 & \textbf{0.86} \\
& Cable & 0.72 & 0.63 & 0.71 & 0.63 & 0.66 & 0.63 & 0.70 & \underline{0.85} & 0.82 & \textbf{0.86} \\
& Capsule & 0.63 & 0.70 & 0.52 & 0.52 & 0.54 & 0.55 & 0.73 & \textbf{0.83} & \underline{0.82} & \textbf{0.83} \\
& Hazelnut & 0.79 & 0.83 & 0.70 & 0.69 & 0.70 & 0.70 & \underline{0.88} & \underline{0.88} & \textbf{0.91} & 0.86 \\
& Metal Nut & 0.52 & 0.54 & 0.51 & 0.54 & 0.54 & 0.53 & 0.58 & 0.57 & \underline{0.65} & \textbf{0.76} \\
& Pill & 0.64 & 0.68 & 0.53 & 0.53 & 0.55 & 0.55 & \underline{0.72} & \textbf{0.74} & 0.70 & 0.71 \\
& Screw & 0.72 & 0.78 & 0.74 & 0.73 & 0.71 & 0.72 & 0.79 & \textbf{0.86} & 0.76 & \underline{0.85} \\
& Toothbrush & 0.73 & 0.82 & 0.62 & 0.61 & 0.55 & 0.57 & 0.75 & \textbf{0.93} & \underline{0.92} & \underline{0.92} \\
& Transistor & 0.56 & 0.60 & 0.53 & 0.54 & 0.51 & 0.52 & 0.63 & \textbf{0.80} & \underline{0.77} & \underline{0.77} \\
& Zipper & 0.60 & 0.67 & 0.57 & 0.57 & 0.57 & 0.58 & 0.65 & \textbf{0.78} & 0.69 & \underline{0.76} \\
\arrayrulecolor{black!60}\cmidrule{2-12}
& Mean & 0.64 & 0.68 & 0.60 & 0.59 & 0.59 & 0.59 & 0.70 & \underline{0.81} & 0.78 & \textbf{0.82} \\
\arrayrulecolor{black!60}\cmidrule{1-12}
& Global mean & 0.63 & 0.70 & 0.60 & 0.60 & 0.60 & 0.60 & 0.70 & \textbf{0.82} & \underline{0.80} & \textbf{0.82} \\
\arrayrulecolor{black}\bottomrule

\end{tabularx}

}
\end{table}
